# Supplementary material for: When is BERT Multilingual? Isolating Crucial Ingredients for Cross-lingual Transfer
Source: arXiv:2110.14782 source file (2022-05-03)
Supplement: Supplementary file 1 [file DiffCorpus.tex]

\begin{table}[t]
\centering
% Uncomment to resize
\resizebox{\linewidth}{!}{
\begin{tabular}{ccccccccc}\toprule
% Header -------------------------------------

% \multirow{2}{*}{\textbf{Type}} & \multicolumn{4}{c}{\supdiff~(Avg. over 4 languages)} \\ \cmidrule(lr){2-5}
\multirow{2}{*}{\textbf{Type}} & \multicolumn{2}{c}{\textbf{XNLI}} & \multicolumn{2}{c}{\textbf{NER}} & \multicolumn{2}{c}{\textbf{POS}} & \multicolumn{2}{c}{\textbf{XQuAD}} \\ \cmidrule(lr){2-3} \cmidrule(lr){4-5} \cmidrule(lr){6-7} \cmidrule(lr){8-9}

% & {\small \textbf{XNLI}} & {\small \textbf{NER}} & {\small \textbf{POS}} & {\small \textbf{XQuAD}} \\ \midrule

% \text{Non-parallel} & \textbf{-5.2} & \textbf{-14.8} & \textbf{-2.0} & \textbf{-5.0}\\ \cdashlinelr{1-5}
% \text{Parallel} & -1.0 & -1.9 & -0.4 & 1.4\\

% \bottomrule

                      & BZ            & \supdiff          & BZ            & \supdiff         & BZ            & \supdiff         & BZ             & \supdiff          \\ \midrule
\textbf{Parallel}              & 69.3          & -1.0              & 83.7          & -1.9             & 95.4          & -0.4             & 61.2           & 1.3               \\ \cdashlinelr{1-9}
\textbf{Non-parallel}  & \multirow{2}{*}{67.4}          & \multirow{2}{*}{-1.8}              & \multirow{2}{*}{80.0}          & \multirow{2}{*}{-4.9}             & \multirow{2}{*}{94.9}          & \multirow{2}{*}{-0.7}             & \multirow{2}{*}{58.6}           & \multirow{2}{*}{-0.6}              \\
\textbf{(Same domain)} & & & & & & & & \\ \cdashlinelr{1-9}
\textbf{Non-parallel}   & \multirow{2}{*}{62.8}          & \multirow{2}{*}{-5.9}              & \multirow{2}{*}{60.4}          & \multirow{2}{*}{-22.0}            & \multirow{2}{*}{91.3}          & \multirow{2}{*}{-4.2}             & \multirow{2}{*}{49.0}           & \multirow{2}{*}{-2.9}              \\
\textbf{(Diff domain)} & & & & & & & & \\
% Non-parallel (250K)   & 62.2          & -5.2              & 68.6          & -14.8            & 93.2          & -2.0             & 48.8           & -5.0              \\
\bottomrule

\end{tabular}
% Uncomment to resize
}
\caption{Results for the \textit{Transliteration} transformation when a bilingual model is pre-trained on parallel and non-parallel corpora~\secref{subsection:diffcorpus}.
The scores are averaged over four languages.
Using a non-parallel corpus inhibits transfer when compared to a parallel corpus.}
\label{table:TransliterationDiff}
\end{table}
